# Supplementary material for: Temporal Graph ODEs for Irregularly-Sampled Time Series
Source: arXiv:2404.19508 source file (2024-04-30)
Supplement: Supplementary file 1 [file appendix.tex]

\section{Appendix}
\subsection{Explored hyper-parameter space}
\label{app:hyperparams}

In Table~\ref{tab:general_configs} %Table~\ref{tab:configs_heat} and Table~\ref{tab:configs_traffic} 
we report the grids of hyper-parameters employed in our experiments by each
method. We recall that the $\epsilon$ hyper-parameter is only used in our method, and that {\it embedding dim} equal to {\it None} means that no encoder and readout are employed.

\input{Tables/general_conf}

\subsection{Software and Hardware}
\label{app:sw_hw}
The Python~\cite{python} code used to run all the computational experiments is available upon acceptance. We relied on the following open-source libraries:
\begin{itemize}
    \item PyTorch~\cite{pytorch};
    \item PyTorch Geometric~\cite{pyg};
    \item Torch Spatiotemporal~\cite{tsl};
    \item Torch Geometric Temporal~\cite{rozemberczki2021pytorch};
    \item NumGraph~\cite{numgraph}.
\end{itemize}
For all the baselines, we run all the experiments by relying on their open-source implementations.

We carried out the experiments on 7 nodes of a cluster with 96 Xeon Gold 6240R CPU @ 2.40GHz per node.
